# Supplementary material for: Learning Implicit Text Generation via Feature Matching
Source: arXiv:2005.03588 source file (2020-05-09)
Supplement: Supplementary file 1 [file appendix_main.tex]

%
% File acl2020.tex
%
%% Based on the style files for ACL 2020, which were
%% Based on the style files for ACL 2018, NAACL 2018/19, which were
%% Based on the style files for ACL-2015, with some improvements
%%  taken from the NAACL-2016 style
%% Based on the style files for ACL-2014, which were, in turn,
%% based on ACL-2013, ACL-2012, ACL-2011, ACL-2010, ACL-IJCNLP-2009,
%% EACL-2009, IJCNLP-2008...
%% Based on the style files for EACL 2006 by 
%%e.agirre@ehu.es or Sergi.Balari@uab.es
%% and that of ACL 08 by Joakim Nivre and Noah Smith

\documentclass[11pt,a4paper]{article}
\usepackage[hyperref]{acl2020}
\usepackage{times}
\usepackage{latexsym}

% This is not strictly necessary, and may be commented out,
% but it will improve the layout of the manuscript,
% and will typically save some space.
\usepackage{microtype}

% inkpad: Added for images/table
\usepackage{graphicx}
\graphicspath{{figures/}}
\usepackage{multirow}
\usepackage{amsmath}
\usepackage{amssymb}

%\aclfinalcopy % Uncomment this line for the final submission
%\def\aclpaperid{2139} %  Enter the acl Paper ID here

%\setlength\titlebox{5cm}
% You can expand the titlebox if you need extra space
% to show all the authors. Please do not make the titlebox
% smaller than 5cm (the original size); we will check this
% in the camera-ready version and ask you to change it back.

\title{Supplementary for Learning Controllable Text Generation By Matching Features from Pre-trained Language Models}

\author{First Author \\
  Affiliation / Address line 1 \\
  Affiliation / Address line 2 \\
  Affiliation / Address line 3 \\
  \texttt{email@domain} \\\And
  Second Author \\
  Affiliation / Address line 1 \\
  Affiliation / Address line 2 \\
  Affiliation / Address line 3 \\
  \texttt{email@domain} \\}

\date{}

\begin{document}
\maketitle
%\begin{abstract}Generative feature matching network (GFMN) is an approach for training state-of-the-art implicit generative models for images by performing moment matching on features from pre-trained neural networks. In this paper, we present new GFMN formulations that are effective for sequential data. Our experimental results show the effectiveness of the proposed method, SeqGFMN, for three distinct generation tasks:%unconditional text generation,
%class-conditional text generation, 
%and unsupervised text style transfer.
%SeqGFMN is stable to train and outperforms various adversarial approaches for text generation and text style transfer.
%\end{abstract}

%\input{introduction} 
%\input{approaches}
%\input{related_work} 
%\input{experiments}
%\input{conclusion}

%\bibliography{anthology,acl2020}
%\bibliographystyle{acl_natbib}

\input{appendix}
\end{document}
